# Supplementary material for: Towards Human-Level Book-Writing Capability
Source: arXiv:2605.17064 source file (2026-06-28)
Supplement: Supplementary file 1 [file evaluation_appendix.tex]

\appendix

\section{Additional Evaluation Material}\label{sec:evaluation-appendix}

This appendix provides supporting material for the evaluation: the first-chapter opening diagnostic slate, pass-rate breakdowns for the deterministic launch-control rows, scaffold-retention breakdowns, score-stability estimates under reruns, and additional details on the judge prompts and deterministic metrics used in the evaluation.

\subsection{First-chapter opening diagnostic slate}\label{sec:evaluation-appendix-xhigh-slate}\label{sec:evaluation-appendix-support}

Table~\ref{tab:writing-quality-diagnostics} aligns the appendix with the diagnostic structure used in the main writing-quality section. The nine rows are split into two groups. The first six rows evaluate narrative development in the opening: whether the chapter turns setup into pressure, sustains problems and goals, keeps larger questions open, and converts obstacles into response. These rows are deterministic early-window checks over the generated first chapter text. The final three rows evaluate narrative clarity: whether the reader can understand the initial situation, track viewpoint, and remain oriented inside the scene. These rows use the prompt-based first-chapter control judge documented in Section~\ref{sec:evaluation-appendix-control-prompts}.

\begin{table}[h]
\centering
\footnotesize

\setlength{\tabcolsep}{4pt}
\begin{tabular*}{0.98\linewidth}{@{\extracolsep{\fill}}p{0.24\linewidth}p{0.20\linewidth}p{0.46\linewidth}}
\toprule
Diagnostic & Evaluation route & What it checks \\
\midrule
Setup becomes live problem & Deterministic launch control & The requested setup develops into a source of narrative pressure rather than remaining only premise, description, or genre frame. \\
Early problem stays active & Deterministic launch control & An early problem continues to shape the unfolding story rather than being resolved immediately or dropped. \\
Same problem stays active & Deterministic launch control & The chapter remains organized around the same underlying problem or a clearly connected transformation of it. \\
Same goal stays active & Deterministic launch control & An early goal, desire, obligation, or inquiry continues to organize later choices and consequences. \\
Blocked goal triggers response & Deterministic launch control & A blocked goal produces a meaningful response that changes the character's situation or what happens next. \\
Mystery remains unresolved & Deterministic launch control & Important questions remain active by the end of the first chapter without becoming arbitrary or merely vague. \\
\addlinespace[0.25em]
Initial situation is clear & Prompt-based control judge & The opening provides enough context to locate the central situation and follow the first scene without static exposition. \\
Viewpoint control holds & Prompt-based control judge & Perceptions, thoughts, knowledge, and judgments remain attributable to a narrator or character. \\
Scene grounding stays legible & Prompt-based control judge & Readers can update where and when the current scene is happening and how it connects to the surrounding narrative. \\
\bottomrule
\end{tabular*}
\caption{First-chapter opening diagnostic slate used in the main writing-quality section. The deterministic rows are reported as pass rates; the three clarity rows use the prompt-based control judge described in Section~\ref{sec:evaluation-appendix-control-prompts}.}
\label{tab:writing-quality-diagnostics}
\end{table}
\FloatBarrier

\subsection{Deterministic launch-control pass rates}\label{sec:evaluation-appendix-launch-control-rates}

Table~\ref{tab:launch-control-pass-rates} reports the deterministic narrative-development rows from the main first-chapter opening evaluation. Each value is a per-prompt pass rate on the shared 360-prompt comparison. These rows are not 1--7 judge scores; they are boolean checks over early chapter windows. The prompt-based clarity rows are documented separately because they are produced by the first-chapter control judge rather than by these deterministic checks.

\begin{table}[h]
\centering
\footnotesize

\setlength{\tabcolsep}{4pt}
\begin{tabular*}{0.82\linewidth}{@{\extracolsep{\fill}}lcc}
\toprule
Diagnostic & Our model & \shortstack{GPT-5.5\\xhigh} \\
\midrule
Setup becomes live problem & 22.2\% & 0.6\% \\
Early problem stays active & 59.2\% & 19.2\% \\
Same problem stays active & 38.9\% & 5.3\% \\
Same goal stays active & 62.8\% & 12.5\% \\
Blocked goal triggers response & 54.4\% & 16.7\% \\
Mystery remains unresolved & 66.9\% & 28.9\% \\
\bottomrule
\end{tabular*}
\caption{Deterministic launch-control pass rates for the narrative-development diagnostics in the first-chapter opening evaluation. The row now titled \emph{Mystery remains unresolved} corresponds to the original metric label \emph{Key questions stay open}; the row now titled \emph{Blocked goal triggers response} corresponds to the original metric label \emph{Blocked goal turns into action}.}
\label{tab:launch-control-pass-rates}
\end{table}
\FloatBarrier

\subsection{Launch-control results by prompt category}\label{sec:evaluation-appendix-gpt-categories}\label{sec:evaluation-appendix-gpt-families}

Table~\ref{tab:writing-quality-category-split} splits the available deterministic launch-control rows into original-fiction and fanfiction prompts. The table keeps only diagnostics that remain part of the revised main first-chapter opening structure.

\begin{table}[h]
\centering
\footnotesize
\setlength{\tabcolsep}{4pt}
\begin{tabular*}{0.95\linewidth}{@{\extracolsep{\fill}}lccc}
\toprule
Slice & \shortstack{Setup becomes\\live problem} & \shortstack{Early problem\\stays active} & \shortstack{Same problem\\stays active} \\
\midrule
Original fiction & 23.3 / 0.4 & 57.9 / 20.0 & 41.2 / 6.7 \\
Fanfiction & 20.0 / 0.8 & 61.7 / 17.5 & 34.2 / 2.5 \\
\bottomrule
\end{tabular*}
\caption{Category-level split for the available deterministic launch-control diagnostics. Each cell reports our model / GPT-5.5 xhigh pass rates in percent.}
\label{tab:writing-quality-category-split}
\end{table}
\FloatBarrier

\subsection{Scaffold-retention breakdowns}\label{sec:evaluation-appendix-genre}

Tables~\ref{tab:storycap-original-genres} and~\ref{tab:storycap-original-vs-fanfiction} expand the main-text scaffold-retention results. The first table breaks original fiction out by genre, and the second restores the usefulness rows for the original-fiction versus fanfiction split. The usefulness rows ask whether an artifact is useful for the next scaffold step, rather than only whether it resembles the requested book.

\begin{table}[h]
\centering
\footnotesize
\setlength{\tabcolsep}{4pt}
\textbf{A. Stage scores}

\vspace{0.25em}

\begin{tabular*}{0.98\linewidth}{@{\extracolsep{\fill}}lcccccc}
\toprule
Genre & \shortstack{Preview\\recog.} & \shortstack{Preview\\useful} & \shortstack{Plan\\recog.} & \shortstack{Plan\\useful} & \shortstack{First chapter\\text recog.} & \shortstack{First chapter\\text useful} \\
\midrule
Fantasy & 6.64 & 4.96 & 3.94 & 2.74 & 3.58 & 3.05 \\
Sci-fi & 6.62 & 5.00 & \textbf{4.20} & 2.67 & 3.25 & 2.77 \\
Romance & 6.50 & 4.65 & 3.40 & 2.30 & 3.35 & 3.20 \\
Mystery & 6.75 & 5.05 & 3.90 & 2.75 & \textbf{3.85} & 3.35 \\
Thriller & 6.80 & 5.15 & 3.55 & 2.50 & 3.50 & 2.70 \\
Historical & 6.60 & 4.90 & 3.80 & 2.50 & 3.20 & \textbf{3.60} \\
Horror & 6.30 & 4.70 & 3.40 & 2.60 & 3.40 & 2.80 \\
Drama & 6.50 & 4.90 & 3.40 & 2.60 & 3.10 & 2.80 \\
Comedy & 6.50 & 4.90 & 3.70 & \textbf{2.80} & 3.40 & 2.60 \\
\bottomrule
\end{tabular*}

\vspace{0.75em}

\textbf{B. Handoff scores}

\vspace{0.25em}

\begin{tabular*}{0.98\linewidth}{@{\extracolsep{\fill}}lccc}
\toprule
Genre & Preview$\rightarrow$Plan & Plan$\rightarrow$first chapter text & Constraints$\rightarrow$first chapter text \\
\midrule
Fantasy & 4.31 & \textbf{3.51} & 3.45 \\
Sci-fi & 4.42 & 3.23 & 3.08 \\
Romance & 3.80 & 3.40 & 3.05 \\
Mystery & 4.40 & 3.45 & \textbf{3.55} \\
Thriller & 4.00 & 2.70 & 3.00 \\
Historical & \textbf{4.50} & 3.50 & 3.50 \\
Horror & 4.30 & 2.90 & 3.20 \\
Drama & 3.80 & 3.40 & 3.10 \\
Comedy & 4.30 & 3.50 & 3.30 \\
\bottomrule
\end{tabular*}
\caption{Original-fiction genre rollup on the 360-prompt benchmark. Columns report Book Preview, Book Plan, first chapter text, and the three handoff rows on the shared 1--7 scale. Bold marks the strongest later-stage or transfer value in each original-fiction genre column.}
\label{tab:storycap-original-genres}
\end{table}

\begin{table}[h]
\centering
\footnotesize
\setlength{\tabcolsep}{5pt}
\textbf{A. Stage scores}

\vspace{0.25em}

\begin{tabular*}{0.92\linewidth}{@{\extracolsep{\fill}}lcccccc}
\toprule
Slice & \shortstack{Preview\\recog.} & \shortstack{Preview\\useful} & \shortstack{Plan\\recog.} & \shortstack{Plan\\useful} & \shortstack{First chapter\\text recog.} & \shortstack{First chapter\\text useful} \\
\midrule
Original fiction & 6.62 & 4.95 & 3.84 & 2.65 & 3.47 & 3.00 \\
Fanfiction & 6.16 & 4.58 & 2.14 & 2.30 & 2.56 & 2.61 \\
\bottomrule
\end{tabular*}

\vspace{0.75em}

\textbf{B. Handoff scores}

\vspace{0.25em}

\begin{tabular*}{0.92\linewidth}{@{\extracolsep{\fill}}lccc}
\toprule
Slice & Preview$\rightarrow$Plan & Plan$\rightarrow$first chapter text & Constraints$\rightarrow$first chapter text \\
\midrule
Original fiction & 4.25 & 3.35 & 3.30 \\
Fanfiction & 2.68 & 2.87 & 2.57 \\
\bottomrule
\end{tabular*}
\caption{Top-level original-fiction versus fanfiction comparison on the 360-prompt benchmark. Panel A reports requested-book recognizability and next-step usefulness at Book Preview, Book Plan, and first chapter text. Panel B reports the three local handoff rows on the same 1--7 scale.}
\label{tab:storycap-original-vs-fanfiction}
\end{table}
\FloatBarrier

\subsection{Score stability under reruns}\label{sec:evaluation-appendix-reliability}

Table~\ref{tab:repeatability-summary} reports the benchmark-level standard deviations obtained by rerunning the shared 1--7 evaluation pipeline. These values summarize the spread of the aggregate scores rather than per-prompt disagreement. Across all rows, the observed rerun spread remains small relative to the main effects in the paper, supporting the interpretation that the reported benchmark-level patterns are stable under reruns.

\begin{table}[h]
\centering
\footnotesize
\setlength{\tabcolsep}{6pt}
\begin{tabular*}{0.95\linewidth}{@{\extracolsep{\fill}}llc}
\toprule
Artifact & Measure & \shortstack{Typical rerun\\spread (SD)} \\
\midrule
Book Preview & Looks like requested book & 0.07 \\
Book Preview & Useful for next writing step & 0.07 \\
Book Plan & Looks like requested book & 0.06 \\
Book Plan & Useful for next writing step & 0.04 \\
First chapter text & Looks like requested book & 0.10 \\
First chapter text & Useful for next writing step & 0.10 \\
\bottomrule
\end{tabular*}
\caption{Score stability of the shared 1--7 benchmark under repeated generation and judging. Each row reports the benchmark-level rerun standard deviation for the corresponding metric.}
\label{tab:repeatability-summary}
\end{table}
\FloatBarrier

\subsection{First-chapter writing-quality scores and GPT baseline generation}
\label{sec:evaluation-appendix-quality-score-computation}

This subsection documents only the nine first-chapter writing-quality scores used in the main comparison. It does not cover the scaffold-retention, book-plan, prompt-following, or long-generation consistency scores.

The nine writing-quality rows use two different evaluation routes. Six rows are deterministic launch-control checks over the generated first-chapter text. These rows do not use an LLM judge prompt. They split the chapter into paragraphs, inspect early paragraph windows, extract shallow narrative cues, and return a binary pass/fail value. The reported score is the pass rate over the matched benchmark prompts. The remaining three rows use a prompt-based first-chapter clarity judge. These rows are scored by a local Gemma judge on a 1--7 scale with three panel passes and median aggregation.

\begin{table}[h]
\centering
\footnotesize

\setlength{\tabcolsep}{4pt}
\begin{tabular*}{0.98\linewidth}{@{\extracolsep{\fill}}p{0.25\linewidth}p{0.22\linewidth}p{0.43\linewidth}}
\toprule
Writing-quality score & Prompt used & Computation \\
\midrule
Setup becomes live problem & No judge prompt; deterministic launch-control check & Uses a preview-specific setup package and checks whether the first 12 chapter paragraphs contain a local question--exchange--constraint window. The row passes when the requested setup becomes an explicit early interaction under pressure rather than remaining only atmospheric or explanatory. \\
Early problem stays active & No judge prompt; deterministic launch-control check & Uses the chapter-only question-to-pressure conversion check in paragraphs 1--12. The row passes when an explicit question is followed by dialogue or interaction in the same or next paragraph, and a concrete constraint or refusal appears soon after. \\
Same problem stays active & No judge prompt; deterministic launch-control check & Uses the goal-update coherence check in paragraphs 1--8. The row first requires an early goal--obstacle--attempt setup in paragraphs 1--4, then checks whether the same burden is still being handled later in the window. \\
Same goal stays active & No judge prompt; deterministic launch-control check & Uses the goal-anchor persistence check in paragraphs 1--12. The row requires an early goal anchor, at least three paragraphs in the window that still serve the same anchored goal frame, and at least one anchored paragraph after the initial launch window. \\
Blocked goal triggers response & No judge prompt; deterministic launch-control check & Uses the goal--obstacle--attempt check in paragraphs 1--4. The row passes when the opening reaches an explicit goal cue, then an obstacle cue, and then an attempted response within that early window. This corresponds to the original code label \emph{Blocked goal turns into action}. \\
Mystery remains unresolved & No judge prompt; deterministic launch-control check & Uses the partial-or-deferred gap check in paragraphs 1--12. The row passes when at least one concrete question remains active through later exchange, constraint, refusal, or handoff rather than collapsing immediately into closure or irrelevance. This corresponds to the original code label \emph{Key questions stay open}. \\
\addlinespace[0.25em]
Initial situation is clear & Gemma first-chapter clarity judge; internal key \texttt{opening\_orientation} & The judge asks whether the opening provides enough who, where, when, and current-pressure framing for a usable situation model without sinking into inert exposition or lore dumping. \\
Viewpoint control holds & Gemma first-chapter clarity judge; internal key \texttt{viewpoint\_control} & The judge asks whether the chapter maintains a coherent relation among narrator, focal character, mental access, knowledge state, and psychic distance, or clearly signals shifts. \\
Scene grounding stays legible & Gemma first-chapter clarity judge; internal key \texttt{scene\_grounding} & The judge asks whether shifts in time, location, scene, flashback, or summary remain legible enough for the reader to stay oriented inside a stable local situation. \\
\bottomrule
\end{tabular*}
\caption{Prompt route and computation method for the nine first-chapter writing-quality scores. The first six scores are deterministic pass/fail checks. The final three scores use the prompt-based Gemma clarity judge.}
\label{tab:first-chapter-quality-score-computation}
\end{table}
\FloatBarrier

\paragraph{Deterministic launch-control rows.}
The deterministic rows are narrow early-chapter checks rather than general literary-quality judgments. The notation \texttt{p1\_4}, \texttt{p1\_8}, and \texttt{p1\_12} means ``within paragraphs 1--4,'' ``within paragraphs 1--8,'' and ``within paragraphs 1--12,'' respectively. The metric code extracts cue families such as explicit questions, dialogue or speech markers, interaction verbs, constraint and refusal cues, goal cues, attempt cues, causal-handoff cues, role or name overlap, place cues, and content-token overlap. Each deterministic row returns a binary pass/fail value for each valid generated chapter. The aggregate score reported in the main writing-quality comparison is the pass rate over the matched prompt set.

\paragraph{Prompt-based clarity rows.}
The three clarity rows use a separate local judge prompt family with \texttt{google/gemma-4-31B-it}. Each chapter is scored independently on a 1--7 scale for each criterion. The setup uses three panel passes and aggregates the panel scores by the median. The judge frame begins as follows:

\begin{quote}
\footnotesize
\begin{verbatim}
You are judging first-chapter narrative quality on a small evidence-first
rubric pack.

Judge only the chapter excerpt shown below.
If an excerpt is truncated, do not invent missing evidence from the unseen
remainder.
Score the chapter independently. Do not reward generic polish if the control
fails.
Do not compare prestige, style preference, or likely popularity. Judge only the
listed dimensions.

Score anchors:
Score 7 = clearly strong, well-supported, and well-integrated.
Score 4 = mixed, partial, or somewhat leaky.
Score 1 = absent, failed, contradictory, or untrackable.
\end{verbatim}
\end{quote}

The prompt then injects the three criteria listed in Table~\ref{tab:first-chapter-quality-score-computation} and requests short evidence-bearing JSON output. A representative output shape is:

\begin{quote}
\footnotesize
\begin{verbatim}
{
  "prompt_id": "...",
  "model_key": "...",
  "metrics": {
    "opening_orientation": {"score": 4,
      "panel_scores": [4, 4, 4], "evidence": "..."},
    "viewpoint_control": {"score": 5,
      "panel_scores": [5, 5, 5], "evidence": "..."},
    "scene_grounding": {"score": 6,
      "panel_scores": [6, 6, 6], "evidence": "..."}
  }
}
\end{verbatim}
\end{quote}

\paragraph{GPT-5.5 xhigh baseline generation.}
The GPT-5.5 xhigh baseline is generated with the same staged comparison harness used for the other external baselines. The benchmark contains 360 prompts. For each prompt, the baseline reuses the same fixed source-book preview as the other models. The GPT baseline therefore does not regenerate the preview. Instead, it generates only the downstream stage-2 artifacts: the book plan, the first-chapter plan, and the first-chapter text. This fixed-preview setup makes the comparison focus on downstream planning and chapter drafting rather than on differences in preview generation.

The GPT-5.5 xhigh run uses OpenAI \texttt{gpt-5.5} with reasoning effort \texttt{xhigh}. Each stage is sent as a fresh provider-chat request rather than as one long multi-turn conversation. The model receives only the original prompt, the fixed source preview, and the previously generated stage artifacts needed for the current step. The generated artifacts are parsed back into the same strict bundle contract before scoring.

The three baseline-generation stages are:

\begin{itemize}
\item \textbf{Book-plan stage.} The model receives the original benchmark request, the fixed source-book preview, and the required stage-2 book-plan tail contract. It is asked to continue from the stage-2 boundary and return only the planning sections that follow the preview.
\item \textbf{First-chapter-plan stage.} The model receives the original prompt, the fixed source preview, the generated book plan, and an explicit first-chapter-plan prefix naming the target chapter. It is asked to continue from that prefix and fill the required chapter-summary and scene-breakdown structure.
\item \textbf{First-chapter-text stage.} The model receives the original prompt, the fixed source preview, the generated book plan, the generated first-chapter plan, and an explicit first-chapter-text prefix. It is asked to continue only the chapter body inside the existing code fence and close that fence correctly.
\end{itemize}

The provider-side stage prompts use short system messages that name the target artifact and forbid commentary, followed by user messages that supply the inputs and output contract. The first-chapter-text system message is:

\begin{quote}
\footnotesize
\begin{verbatim}
You write Stage-2 first-chapter text continuations. Return only the continuation
text after the provided prefix. Do not repeat the prefix. Do not explain your
reasoning. Do not add commentary before or after the continuation.
\end{verbatim}
\end{quote}

The user-side stage contracts include the following representative substrings:

\begin{quote}
\footnotesize
\begin{verbatim}
Book-plan stage:
"Expand the stage-1 source book preview into the remaining stage-2 planning
sections."
"Return only these sections, starting exactly at `## World Rules`:"
## World Rules
## Short Story Arcs
## Character Archetypes
## Writing Style
## Medium Story Arcs
## Long Story Arcs
## Number of Chapters
## Chapter Names
## Chapters Embedding Space
## Chapters Word Count
"Do not repeat `## Book Highlight`, `## Book Title`, `## Book Tags`, or
`## Book Archetype`."
"Use the exact section order."
"Each arc section must contain exactly `Arc 1` through `Arc 4`."

First-chapter-plan stage:
"Continue the first chapter plan for the existing Stage-2 bundle."
"Return only the continuation text beginning with the narrative focuses names."
"Your continuation must follow this exact structure:"
<focus name>[; <focus name>...]
**Chapter Summary:**
- <beat>
- <beat>
### Scene Breakdown
#### Scene 1: <title>
**Word Count:** <positive integer>
**Embedding Space:** ...
**Narrative Focus:** ...
**Narrative Perspective:** ...
**Scene Summary:**
- <beat>
- <beat>
"Return only the continuation text after the prefix, not the prefix itself."
"Use exactly `**Chapter Summary:**` and `### Scene Breakdown`."
"Use one or more `#### Scene N:` sections in ascending order."

First-chapter-text stage:
"Continue the first chapter text for the existing Stage-2 bundle."
"Return only the chapter body that belongs inside the code fence, and then close
the fence with ``` on its own line."
"Write chapter prose only."
"Do not add any text after the closing fence."
\end{verbatim}
\end{quote}

All GPT-5.5 xhigh outputs are scored with the same downstream scoring stack as the other model outputs. The external-provider runs use non-streaming chat completions with no tool calls and no image inputs. No \texttt{top\_p}, \texttt{top\_k}, or seed overrides are supplied by the harness. Transport-level failures are retried without changing the prompt content. If a chat API stops because of length, the harness appends a continuation request containing the trailing visible excerpt and asks the model to continue exactly from that point. If the merged artifact still fails to parse or the first-chapter text fails to close its fence, the row is rejected for that attempt and does not enter scoring as a valid bundle.

\FloatBarrier
